# Supplementary material for: Stereoscopic Dark Flash for Low-light Photography
Source: arXiv:1901.01370 source file (2019-01-09)
Supplement: Supplementary file 1 [file appendix.tex]

\subsection{Hardware components and specifications}
Below is a complete list of components used in our prototype. The label of each hardware element matches that of Figure \ref{fig:setup}(b):
% \begin{enumerate}[label=\Alph*.]
% \item RGB camera: Camera (FLIR BFS-U3-51S5C-C) + \\ 1/1.8" 4-15.2mm f1.5 lens (Fujinon DV3.8x4SR4A-SA1) + \\ UV/IR cut-off filter (Edmund Optics 89-800) + \\ 435nm cut-on filter (Newport FSQ-GG435)
% \item NIR-G-NUV camera: Camera (FLIR BFS-U3-51S5C-C) with IR-cut filter removed + \\ 1/1.8" 4-15.2mm f1.5 lens (Fujinon DV3.8x4SR4A-SA1)
% \item NIR flash: 740nm LED (QT Brightek QBHP684-IR4BU) +  \\ 
% 715nm cut-on filter (Newport 10CGA-715) 
% \item NUV flash: 395nm LED (Everlight Electronics EAUVA35352GH8)\\
% + 400nm cut-off filter (Edmund Optics 47-285)
% \item White flash: LED Engin LZ4-V4MDPB-0000
% \item Others: sync board by Teensy 3.2, LED driver board by MOSFET, and power by 9v batteries
% \end{enumerate}

\begin{enumerate}[label=\Alph*.]
\item RGB camera:
  \begin{itemize}
    \item Camera (FLIR BFS-U3-51S5C-C)
    \item 1/1.8" 4-15.2mm f1.5 lens (Fujinon DV3.8x4SR4A-SA1)
    \item UV/IR cut-off filter (Edmund Optics 89-800)
    \item 435nm cut-on filter (Newport FSQ-GG435)
  \end{itemize}
\item NIR-G-NUV camera:
  \begin{itemize}
    \item Camera (FLIR BFS-U3-51S5C-C) with IR-cut filter removed 
    \item 1/1.8" 4-15.2mm f1.5 lens (Fujinon DV3.8x4SR4A-SA1)
  \end{itemize}
\item NIR flash:
  \begin{itemize}
	\item 740nm LED (QT Brightek QBHP684-IR4BU)
	\item 715nm cut-on filter (Newport 10CGA-715)
  \end{itemize}
\item NUV flash:
  \begin{itemize}
    \item 395nm LED (Everlight Electronics EAUVA35352GH8)
	\item 400nm cut-off filter (Edmund Optics 47-285)
  \end{itemize}
\item White flash: LED Engin LZ4-V4MDPB-0000
\item Others:
  \begin{itemize}
	\item sync board by Teensy 3.2
    \item LED driver board by MOSFET
    \item power by 9v batteries
  \end{itemize}
\end{enumerate}
The camera has a resolution of $2448 \times 2048$, with a gain range of $0$ to $47$ dB, an exposure time range $6\mu$s to $30$s, and a 12-bit ADC. The interval between adjacent frames is $\max(\mathrm{exposure\_time}, 40\mathrm{ms})$ where $40\mathrm{ms}$ is the time it takes to read and saving and image to our laptop's disk. When we capture dataset in a low-light environment, the exposure time usually ranges from $60\mathrm{ms}$ to $120\mathrm{ms}$, and thus there is no gap between the frames in our burst. We fix the gamma of the cameras to 1, turn off auto white balance, and set our red:green:blue gains to be 1:1:1.

We choose the LEDs and optical filters to achieve the goals that (1) when flashes are on, the RGB camera should have no response and the NUV-G-NIR camera should have a very high response, and (2) the LEDs can emit a small amount of visible light, to allow humans to see when the flashes are on for safety's sake.
We choose off-the-shelf components to approximate the goals where the second goal conflicts with the first one a little bit.
To let NIR-G-NUV camera has high response, NUV flash should be close to 400nm and NIR flash should be close to 700nm, but LED has some spectrum bandwidth which extends to visible part; if too close, the RGB camera also has response.
Eventually we chose to use 740nm and 395nm LEDs with filters to remove the visible component of their emitted light.
Because our NIR-G-NUV camera has low response to UV light, we choose a 395nm LED whose spectrum peak is very close to the extents of visible light.
We used a 435nm cut-on filter in front of the RGB camera to reject blue light from the NUV LED.
The RGB camera uses another filter to reject NIR and NUV light.
Our tests show that, though the RGB camera uses two filters and the NUV-G-NIR camera's lens's IR-cut filter is removed, both cameras have sufficient and comparable ability to focus on the subject of the scene. Figure~\ref{fig:setup}(b) shows the spectrum curves of our final system.
% actually this curve is approximate. I don't know the spectrum distribution of the camera beyond visible region, and the lens' response. 
% \begin{figure} 
% 	\center
% 	\includegraphics[width=0.4\textwidth]{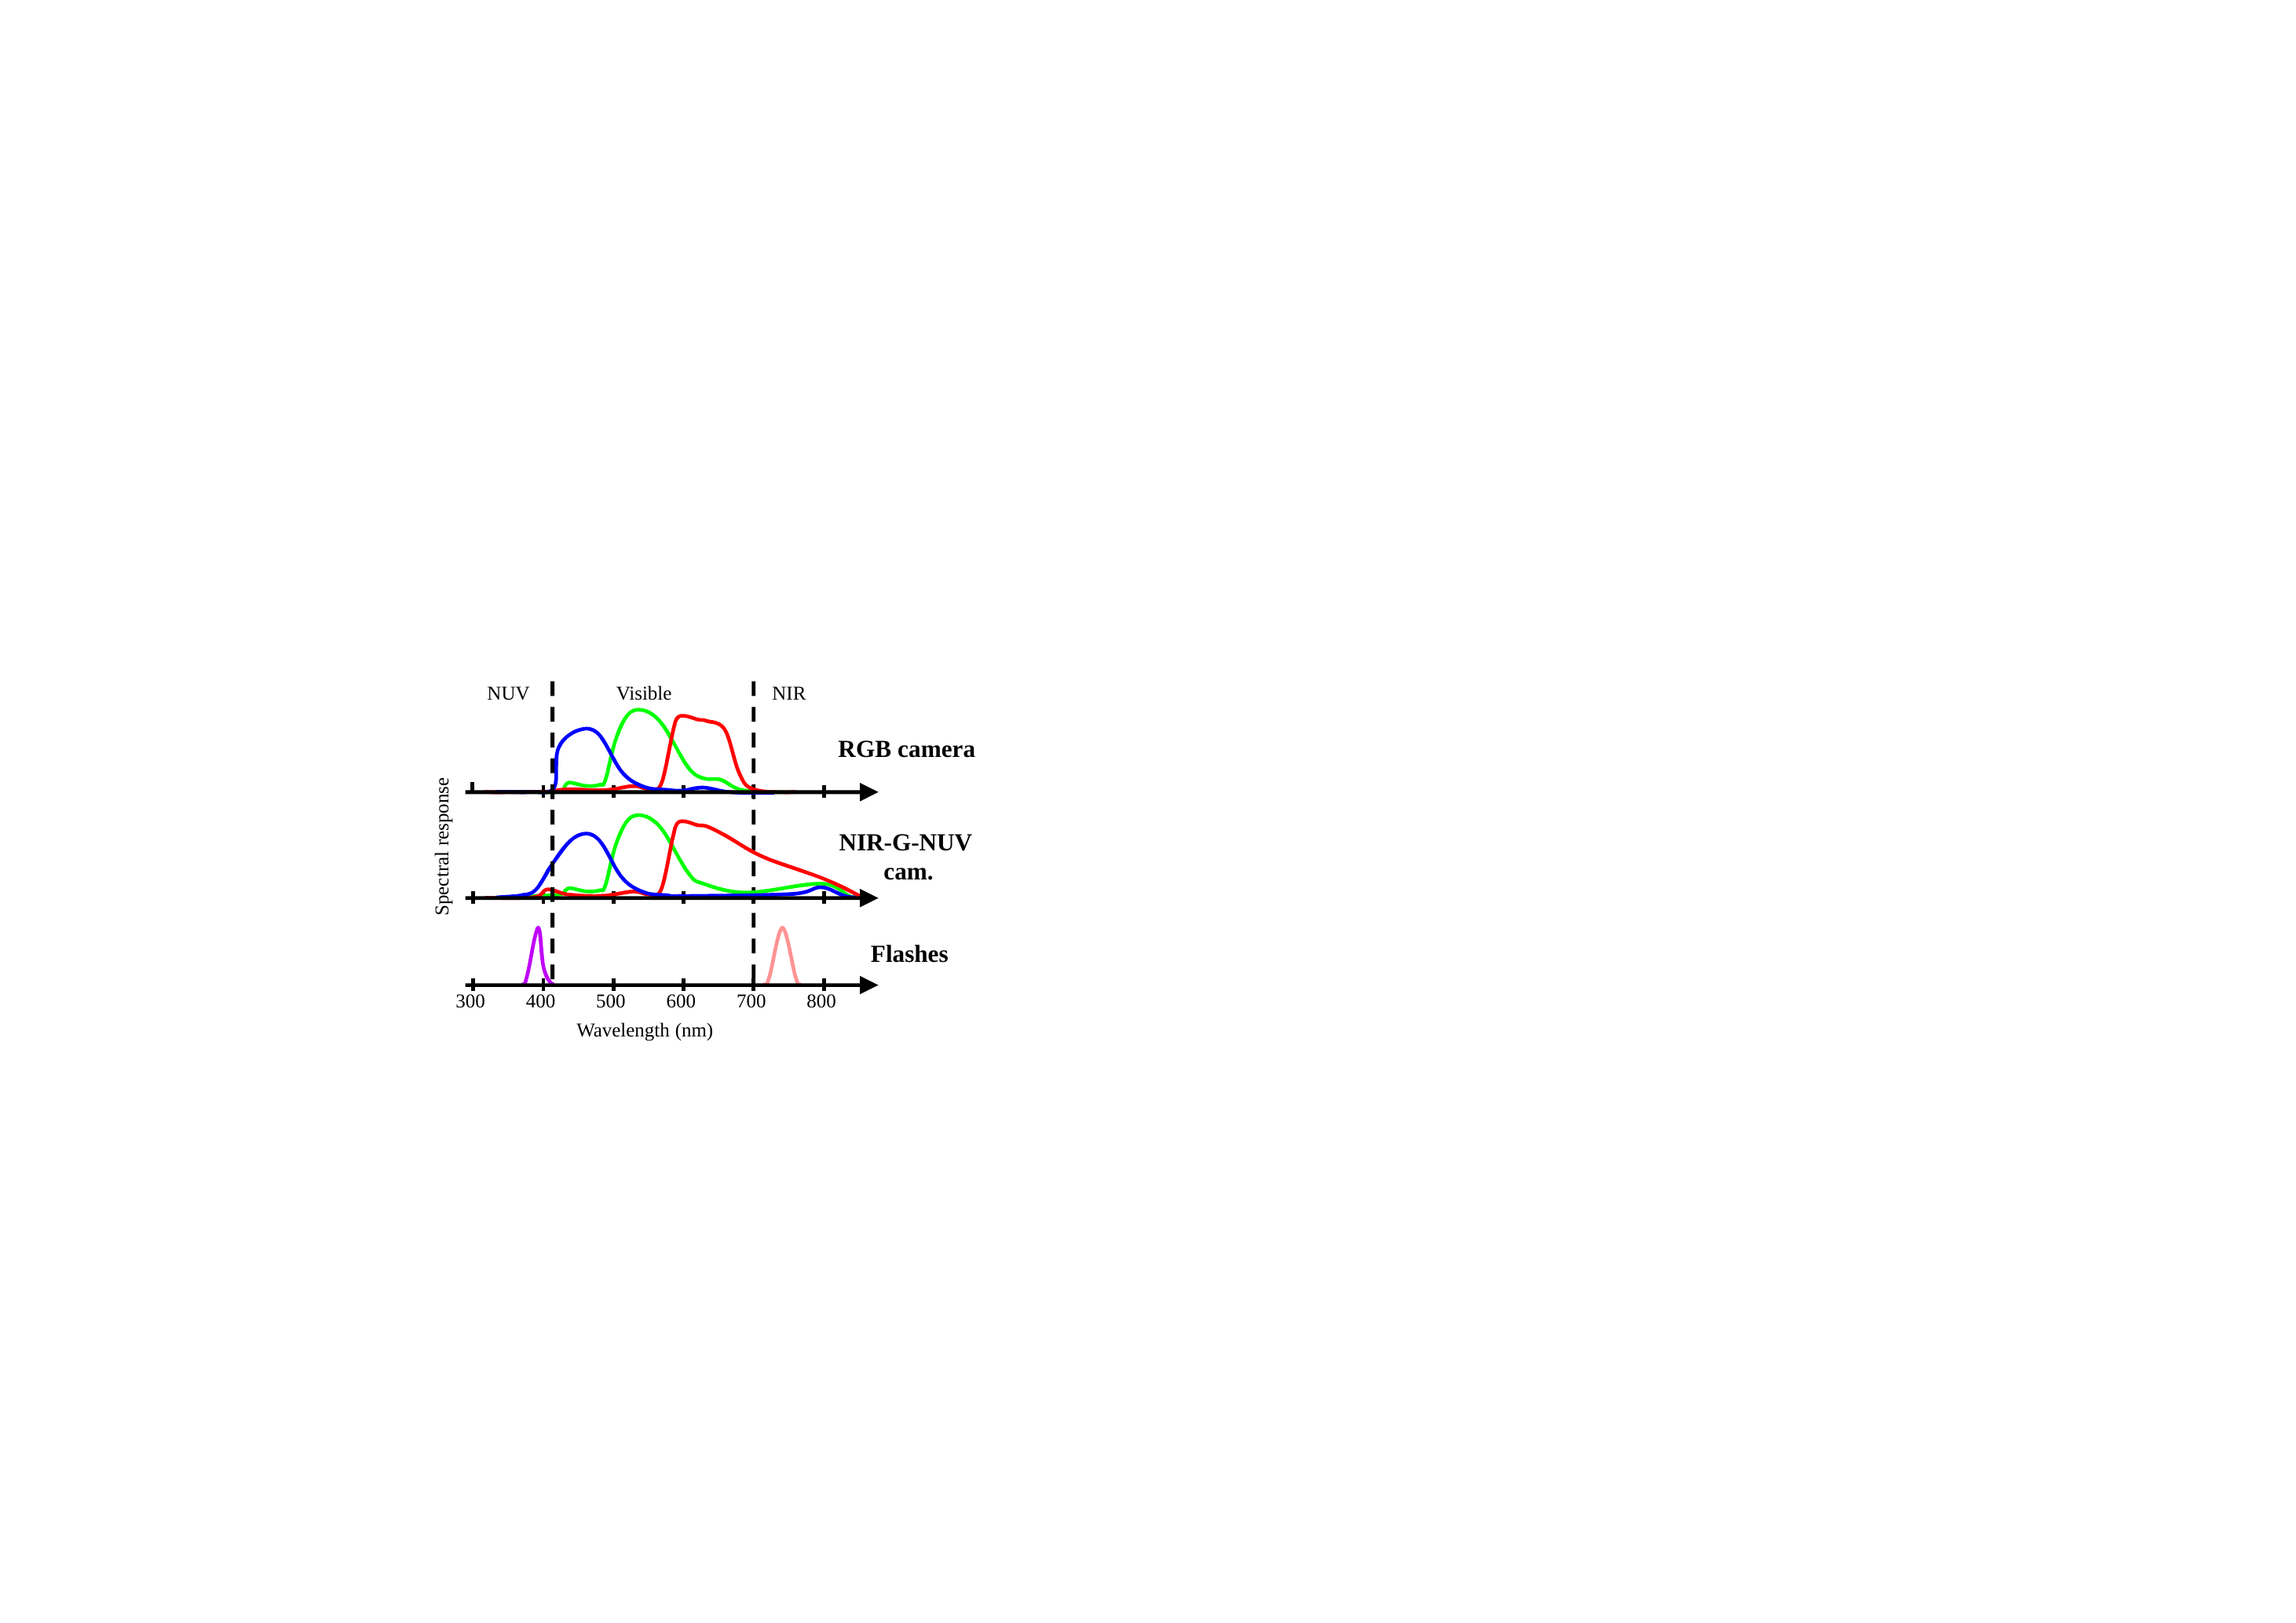}\\
% 	\caption{Spectrum response of the two cameras and spectrum distribution of the two flashes in our hardware prototype with use of off-the-shelf components. Notice that NUV range shifts to the right a little bit.}
% 	\label{fig:practical_spectrum}
% \end{figure}

\subsection{Automatic exposure algorithm}
Most consumer cameras feature an automatic exposure (AE) system to assist in estimating an exposure time and a gain (ISO) that best makes use of a sensor's dynamic range relative to scene irradiance (while also ensuring that most scene content is neither under- nor over-exposed).
Even in the absence of a variable lens aperture and a flash, AE is already a challenging 2D optimization problem in which one must trade off noise with motion blur in a short amount of time.
With two cameras this becomes a more difficult 4D problem, and
the introduction of ``dark" flash with an independent exposure time and gain control brings us to a challenging 6D optimization problem.

To make this problem tractable we constrain our search space significantly. We first require that the two cameras' exposure times match, because doing otherwise may induce motion blur and would make stereo matching unnecessarily challenging. We also fix our dark flash to emit its maximum power, as there is little advantage to illuminating the subject for a longer duration and introducing more blur when the flash is within the eye safety limit.

Our overall AE sequence is as follows:
\begin{enumerate}
\item We find an exposure time $T$ for \camone while fixing its gain to its maximum value of $47$dB, with the flash off.
\item We find a gain for \camtwo while fixing its exposure time to $T$, also with the flash off.
\item We find gains for \camone and \camtwo with white flash, IR flash, and UVIR flashes enabled respectively, while fixing the exposure time to $T$.
\item We compute gains for a fractional flash (recall that in burst 1 and burst 2, there are cases where the flash time is a fraction of $T$).
\item We compute an exposure time and gain for our long exposure time image pair.
\end{enumerate}
Let us describe the details for each step. In (1), on shutter release we first set \camone's gain to its maximum value and set $T$ to $1ms$, and then capture a 16-bit raw image.
We then find the pixel value $v$ at the 99th percentile of the image and compute an approximate inverse gain $r = 50000 / (v+1000)$ (where $50000$ is a large value that is near the limit of a 16 bit sensor, and the $+1000$ term avoid division by small values). 
Next we set the exposure time to be $rT$ and capture the image again, under the assumption that this newly acquired image will have a 99th percentile value that is near $50000$.
We iterate this process until the difference between the old and new exposure times is smaller than $1ms$.
%If the scene is extremely dark ($v<1000$), then the initial value of r is very big and unreliable (the entire histogram is close to clipped). In that case, we set r = 50000/(1000+v) as appropriate.
%
We use this exposure time for all future settings except the long exposure acquisition. 

In (2) and (3), we use this fixed exposure time to search for the gains to apply to \camtwo without a flash, and \camone and \camtwo with a white flash, an IR flash, and a UVIR flash. This is done with the same procedure as described previously, iteratively identifying a gain such that the 99th percentile pixel value is approximately $50000$.

The results of this metering process under different settings are typically (Figure \ref{fig:AE} shows one example): 
\begin{itemize}
\item Without flash, \camone's gain is 47dB and \camtwo's gain is between 40dB and 47dB respectively (\camtwo's gain is smaller because \camtwo receives some infrared light from the environment).
\item With an infrared flash, \camone and \camtwo's gains are about 40dB and less than 5dB respectively (\camone's gain drops from 47dB to 40dB because the infrared flash emits a little bit of red light).
\item With UVIR flashes, the gains depend on how strong the fluorescent light is. If there is little or no fluorescence, gains are similar to those under infrared flash (because \camtwo has a lower response to UV than IR and UV only influences the blue channel, turning on the UV flash based on the IR flash will change the gain very little). If there is fluorescence, gains will be determined by the excited blue light.
\end{itemize}

\begin{figure} 
	\center
	\includegraphics[width=0.5\textwidth]{figures/AE.pdf}\\
	\caption{Automatic exposure algorithm on a toy scene.}
	\label{fig:AE}
\end{figure}

In (4), we use these previously computed metering results to algebraically compute the gains for the fractional flashes in burst 1 and 2 for our two cameras.
In burst 2, that gain for the $1/n$ flash is simply $n$ times the full flash's gain.
In burst 1, the calculation is nontrivial. Suppose the exposure time is $T$, the gain without the flash is $g_e$, the gain with the flash is $g_{ef}$. We must then determine what the gain should be when the flash time is $T/n$. Assuming that the 99th percentile pixel value happens at the same location in all images, we have two equations:
\begin{align}
T g_e L_e &= 50000 \\
T g_{ef} (L_e+L_f) &= 50000
\end{align}
Where $L_e$ and $L_f$ are the intensity of the environment light and the flash light, respectively. The solution to this system of equations is:
\begin{equation}
\hat{g}= {n g_e \over n + g_{e}/g_{ef} - 1}
\end{equation}

To allow us to better simulate the noisier sensor readings we should expect in a standard smart phone camera, we capture additional data in which we use digital gain to increase the noise level of our images.
We capture another three sets of images with exposure times of $\nicefrac{T}{3}$, $\nicefrac{T}{5}$, and $\nicefrac{T}{7}$. We account for these reduced exposure times by increasing the gains of the flash images of \camtwo increase by $3$, $5$, and $7$, respectively.
% Here the unit of gains above is in times, and we next change to dB by $20\log(\cdot)$ for camera settings.

\barron{I don't know what is happening here:}
In (5), suppose without flash, gain of $cam_i$ is $g_i$, i = 1, 2.
%gains of \camone and \camtwo are $g_1=47$dB$=10^{47/20}=224$ and $g_2$, respectively. 
The long exposure time $\tau_i$ will be $\min(10^{g_i/20}T, 30s)$ and gain will be $10^{g_i/20}T / \tau_i$ since both cameras' longest exposure time is 30s.

This auto-exposure approach works well in practice on our dataset, though our images consist of mostly static subjects. In practice, adapting a metering algorithm to moving subjects would require a more sophisticated algorithm that is biased towards shorter exposures, to combat hand or scene motion.
